# Supplementary material for: $\sigma$-zero: Gradient-based Optimization of $\ell_0$-norm Adversarial Examples
Source: arXiv:2402.01879 source file (2025-03-06)
Supplement: Supplementary file 1 [file 2.5k_cifar.tex]

\begin{table}[htbp]
\caption{Fixed budget comparison results with $N=2500$ on CIFAR10. See the caption of Table~\ref{tab:1k_remaining_maximum_budget_cifar} for further details.}
\label{tab:2.5k_maximum_budget_cifar}
\resizebox{\textwidth}{!}{%

\begin{tabular}{c|c|ccc|c|c|ccc|c}
\toprule
\multicolumn{1}{c}{\textbf{Attack}} & \multicolumn{1}{c}{\textbf{M}} & \multicolumn{1}{c}{\textbf{ASR$_{24}$}} & \multicolumn{1}{c}{\textbf{ASR$_{50}$}} & \multicolumn{1}{c}{\textbf{ASR$_{100}$}} & \multicolumn{1}{c}{\textbf{q}} & \multicolumn{1}{c}{\textbf{M}} & \multicolumn{1}{c}{\textbf{ASR$_{24}$}} & \multicolumn{1}{c}{\textbf{ASR$_{50}$}} & \multicolumn{1}{c}{\textbf{ASR$_{100}$}} & \multicolumn{1}{c}{\textbf{q}} \\

\hline

\PGDlzero & \multirow{5}{*}{\carmonshort} & 37.95 & 61.03 & 88.26 & 5.0  & \multirow{5}{*}{\standardshort} & 68.99 & 90.26 & 98.65 & 5.0  \\%
Sparse-RS &  & \textbf{79.41} & 92.97 & 97.57 & 1.5 &  & \textbf{99.91} & 99.98 & 100.0 & 0.1  \\%
\SPGDproj &  & 68.57 & 91.78 & 99.61 & 1.7 &  & 98.49 & 100.0 & 100.0 & 0.13  \\%
\SPGDunproj &  & 69.75 & 92.04 & 99.98 & 1.69 &  & \textbf{99.91} & 100.0 & 100.0 & 0.03  \\%
\cdashline{1-11} \rc\sigmazero &  & 79.25 & \textbf{96.11} & \textbf{99.99} & 5.0 &  & 99.69 & 100.0 & 100.0 & 5.0  \\ \hline%

\PGDlzero & \multirow{5}{*}{\augustinshort} & 32.78 & 59.59 & 89.46 & 5.0 & \multirow{5}{*}{\engstromshort} & 38.22 & 68.75 & 95.56 & 5.0  \\%
Sparse-RS &  & 66.57 & 86.6 & 96.28 & 2.2 &  & 72.34 & 91.30 & 98.37 & 1.9  \\%
\SPGDproj &  & 61.98 & 90.38 & 99.71 & 2.0 &  & 75.77 & 97.73 & 100.0 & 1.2  \\%
\SPGDunproj &  & 67.06 & 94.19 & 99.94 & 1.78  &  & \textbf{83.18} & 99.3 & 100.0 & 0.9 \\%
\cdashline{1-11} \rc\sigmazero &  & \textbf{77.0} & \textbf{98.16} & \textbf{100.0} & 5.0 &  & 83.15 & \textbf{99.36} & 100.0 & 5.0 \\ \hline%

\PGDlzero & \multirow{5}{*}{\croceloneshort} & 22.98 & 36.62 & 68.09 & 5.0& \multirow{5}{*}{\xushort} & 31.45 & 53.05 & 80.9 & 5.0 \\
Sparse-RS &  & 35.54 & 52.97 & 73.27 & 3.5 &  & 75.79 & 87.08 & 93.32 & 1.7 \\
\SPGDproj &  & 33.22 & 62.3 & 95.25 & 3.4 &  & 64.09 & 86.04 & 97.58 & 2.0 \\
\SPGDunproj &  & 36.83 & 71.06 & 98.24 & 3.2 &  & 66.17 & 89.66 & 98.99 & 1.9 \\
\cdashline{1-11} \rc\sigmazero &  & \textbf{40.42} & \textbf{75.16} & \textbf{98.78} & 5.0 &  & \textbf{82.10} & \textbf{97.71} & \textbf{99.98} & 5.0 \\ \hline

\PGDlzero & \multirow{5}{*}{\jiangloneshort} & 34.21 & 44.84 & 68.62 & 5.0 & \multirow{5}{*}{\addepallishort} & 38.73 & 62.75 & 90.00 & 5.0 \\
Sparse-RS &  & 52.88 & 68.35 & 82.48 & 2.6 &  & 72.71 & 88.20 & 95.83 & 1.9 \\
\SPGDproj &  & 52.07 & 78.74 & 98.57 & 2.5&  & 63.33 & 87.84 & 99.37 & 2.0 \\
\SPGDunproj &  & \textbf{56.81} & \textbf{85.42} & \textbf{99.66} & 2.22 &  & 67.23 & 92.05 & 99.87 & 1.76 \\
\cdashline{1-11} \rc\sigmazero &  & 56.61 & 83.80 & 99.25 & 5.0  &  & \textbf{76.16} & \textbf{95.22} & \textbf{99.89} & 5.0 \\ \hline
\end{tabular}

}
\end{table}
