# Supplementary material for: $\sigma$-zero: Gradient-based Optimization of $\ell_0$-norm Adversarial Examples
Source: arXiv:2402.01879 source file (2025-03-06)
Supplement: Supplementary file 2 [file 2.5k_imagenet.tex]

\begin{table}[htbp]
\caption{Fixed budget comparison results with $N=2500$ on ImageNet. See the caption of Table~\ref{tab:1k_maximum_budget_imagenet} for further details.}
\label{tab:2.5k_maximum_budget_imagenet}
\resizebox{\textwidth}{!}{%
  \setlength\tabcolsep{15pt}

\begin{tabular}{c|c|c|c|c|c|c}
\toprule
\multicolumn{1}{c}{\textbf{Attack}} & \multicolumn{1}{c}{\textbf{M}} & \multicolumn{1}{c}{\textbf{ASR$_{150}$}} & \multicolumn{1}{c}{\textbf{q}} & \multicolumn{1}{c}{\textbf{M}} & \multicolumn{1}{c}{\textbf{ASR$_{150}$}} & \multicolumn{1}{c}{\textbf{q}} \\ \hline

Sparse-RS & \multirow{4}{*}{\resnetvulnerableshort} & 95.0 & 0.6 & \multirow{4}{*}{\debenedettishort} & 51.7 & 2.7 \\%
\SPGDproj &  & 99.3 & 0.1 &  & 77.1 & 1.3 \\%
\SPGDunproj &  & 98.3 & 0.1 &  & 77.5 & 1.2 \\%
\cdashline{1-7} \rc\sigmazero &  & \textbf{100.0} & 5.0 &  & \textbf{87.8} & 5.0 \\ \hline

Sparse-RS & \multirow{4}{*}{\engstromimagenetshort} & 86.9 & 1.0 & \multirow{4}{*}{\wongshort} & 90.0 & 0.7 \\
\SPGDproj &  & 91.7 & 0.5 &  & 95.5 & 0.3 \\
\SPGDunproj &  & 89.4 & 0.6 &  & 93.4 & 0.4 \\
\cdashline{1-7} \rc\sigmazero &  & \textbf{97.3} & 5.0&  & \textbf{98.4} & 5.0 \\ \hline

Sparse-RS & \multirow{4}{*}{\hendrycksshort} & 77.6 & 1.6 & \multirow{4}{*}{\salmanshort} & 92.3 & 0.6 \\
\SPGDproj &  & 94.3 & 3.4 &  & 96.5 & 0.3 \\
\SPGDunproj &  & 92.9 & 0.4 &  & 94.4 & 0.3 \\
\cdashline{1-7} \rc\sigmazero  &  & \textbf{99.7} & 5.0 &  & \textbf{99.1} & 5.0 \\ 

\bottomrule
\end{tabular}

}
\end{table}
