# Supplementary material for: $\sigma$-zero: Gradient-based Optimization of $\ell_0$-norm Adversarial Examples
Source: arXiv:2402.01879 source file (2025-03-06)
Supplement: Supplementary file 3 [file 2.5k_mnist.tex]

\begin{table}[htbp]
\caption{Fixed budget comparison results with $N=2500$ on MNIST. See the caption of Table~\ref{tab:1k_remaining_maximum_budget_cifar} for further details.}
\label{tab:2.5k_maximum_budget_mnist}
\resizebox{\textwidth}{!}{%

\begin{tabular}{c|c|ccc|c|c|ccc|c}
\toprule
\multicolumn{1}{c}{\textbf{Attack}} & \multicolumn{1}{c}{\textbf{M}} & \multicolumn{1}{c}{\textbf{ASR$_{24}$}} & \multicolumn{1}{c}{\textbf{ASR$_{50}$}} & \multicolumn{1}{c}{\textbf{ASR$_{100}$}} & \multicolumn{1}{c}{\textbf{q}} & \multicolumn{1}{c}{\textbf{M}} & \multicolumn{1}{c}{\textbf{ASR$_{24}$}} & \multicolumn{1}{c}{\textbf{ASR$_{50}$}} & \multicolumn{1}{c}{\textbf{ASR$_{100}$}} & \multicolumn{1}{c}{\textbf{q}} \\
\hline
\PGDlzero & \multirow{5}{*}{\smallcnnddnshort} & 74.13 & 99.89 & 100.0 & 5.0 & \multirow{5}{*}{\smallcnntradesshort} & 64.08 & 95.51 & 99.2 & 5.0 \\
Sparse-RS &  & 85.67 & 98.6 & 99.97 & 1.5 &  & \textbf{99.71} & 99.95 & 100.0 & 0.3 \\
\SPGDproj &  & 75.47 & 99.00 & 100.0 & 1.0 &  & 78.5 & 99.67 & 99.97 & 1.71 \\
\SPGDunproj &  & 85.58 & 99.83 & 100.0 & 1.9 &  & 69.79 & 99.12 & 99.99 & 1.96 \\
\cdashline{1-11} \rc\sigmazero &  & \textbf{86.99} & \textbf{99.99} & 100.0 & 5.0 &  & 99.19 & \textbf{100.0} & 100.0 & 5.0 \\  \bottomrule
\end{tabular}
}
\end{table}
