# Supplementary material for: $\sigma$-zero: Gradient-based Optimization of $\ell_0$-norm Adversarial Examples
Source: arXiv:2402.01879 source file (2025-03-06)
Supplement: Supplementary file 6 [file pseudo_algorithm.tex]

%\vspace{-2em}
\begin{algorithm}[htb]
  \SetAlgoLined
\DontPrintSemicolon
\footnotesize{
  \KwInput{$\vct x\in [0,1]^d$; y; $\vct\theta$; N; $\eta_0=1.0$; $\sigma=10^{-3}$; $\tau_0=0.3$; $t=0.01$; \textcolor{red}{$k$, the fixed budget limit.}}
  \KwOutput{$\vct x^\star$, the minimum \lzero-norm adversarial example.}
  $\boldsymbol{\delta} \leftarrow \vct 0$; $\quad \vct\delta^\star \leftarrow \vct \infty$; $\quad \tau \leftarrow \tau_0$; $\quad \eta \leftarrow \eta_0$  

   %$\vct\delta^\star \leftarrow \vct\delta$ \label{line:init_optimal}

    \For{i {\rm in} $1, \dots, N$} {

        $\nabla\vct{g} \leftarrow \nabla_{\vct\delta}[\set{L}(\vct x + \vct \delta, y, \vct \theta) + \frac{1}{d}\lzerohat(\vct\delta, \sigma)]$
         
        $\nabla\vct{g} \leftarrow {\nabla\vct{g}}/{\|\nabla\vct{g}\|_\infty}$

        $\vct\delta \leftarrow$ \texttt{clip}$(\vct x + [\vct\delta - \eta\cdot\nabla\vct{g}]) - \vct x$

        $\vct\delta \leftarrow \Pi_\tau(\vct\delta)$ 
        
        $\eta = \texttt{cosine\_annealing}(\eta_0, i)$

        \rm \textbf{if} {$\set{L}(\vct x + \vct \delta, y, \vct \theta) \leq 0$}:
        { $\tau += t\cdot \eta$, {\rm \textbf{else} $\tau -= t\cdot \eta$}} 

        \rm \textbf{if} {$\set{L}(\vct x + \vct \delta, y, \vct \theta) \leq 0 ~\wedge ~ \|\vct\delta\|_0< \|\vct\delta^\star\|_0$}: 
        {  $\vct\delta^\star \leftarrow \vct\delta$}

        \textcolor{red}{\rm \textbf{if} {$\|\vct\delta^\star\|_0 \leq k$}: 
        {  \KwRet{$\vct x^\star \leftarrow \vct x + \vct \delta^\star$}\label{line:early-stop}}\tcp*{\footnotesize{early stopping}}}

        }

        \rm \textbf{if} {$\set{L}(\vct x + \vct \delta^\star, y, \vct \theta) > 0$:}{ { $\vct\delta^\star \leftarrow \infty$}
        
        }

    \KwRet{$\vct x^\star \leftarrow \vct x + \vct \delta^\star$}
    }
\caption{\sigmazeroES Attack Algorithm.}
\label{alg:sigma-zero-ES}
\end{algorithm}
