# Supplementary material for: $\sigma$-zero: Gradient-based Optimization of $\ell_0$-norm Adversarial Examples
Source: arXiv:2402.01879 source file (2025-03-06)
Supplement: Supplementary file 8 [file backup_full_1k_imagenet.tex]

\begin{table*}[t]
\centering
\caption{Fixed budget comparison results with 1000 steps on ImageNet. \revision{Sparse-RS was executed with double the steps, 2000, to ensure fair comparison as it lacks backward passes.} For each attack, we report the corresponding ASR with feature budget level equal to 150.}
\label{tab:maximum_confidence_imagenet_1000}
\resizebox{0.8\textwidth}{!}{%
%\setlength\tabcolsep{8.pt}
\renewcommand{\arraystretch}{1.1}
\begin{tabular}{c|c|c|c|c|c|c}
\hline
Attack & Model & ASR$_{150}$ & q \tiny{(x1000)} & Model & ASR$_{150}$ & q \tiny{(x1000)} \\ \hline
Sparse-RS & \multirow{4}{*}{\resnetvulnerableshort} & 91.5 & 0.34 & \multirow{4}{*}{\salmanshort} & 89.2 & 0.32 \\
sPGD$_{proj}$ &  & 98.5 & 0.04 &  & 95.2 & 0.12 \\
sPGD$_{unproj}$ &  & 97.8 & 0.05 &  & 94.0 & 0.14 \\
\cdashline{1-7} \sigmazero &  & \textbf{100.0} & 2.00 &  & \textbf{98.8} & 2.00 \\ \hline
Sparse-RS & \multirow{4}{*}{\engstromimagenetshort} & 84.1 & 0.49 & \multirow{4}{*}{\hendrycksshort} & 72.2 & 0.77 \\
sPGD$_{proj}$ &  & 91.2 & 0.2 &  & 93.4 & 0.16 \\
sPGD$_{unproj}$ &  & 88.7 & 0.2 &  & 92.1 & 0.17 \\
\cdashline{1-7} \sigmazero &  & \textbf{97.0} & 2.00 &  & \textbf{99.3} & 2.00 \\ \hline
Sparse-RS & \multirow{4}{*}{\wongshort} & 87.5 & 0.35 & \multirow{4}{*}{\debenedettishort} & 47.4 & 1.15 \\
sPGD$_{proj}$ &  & 94.5 & 0.13 &  & 74.9 & 0.55 \\
sPGD$_{unproj}$ &  & 92.6 & 0.16 &  & 76.0 & 0.51 \\
\cdashline{1-7} \sigmazero &  & \textbf{98.2} & 2.00 &  & \textbf{86.2} & 2.00 \\ \hline
\end{tabular}
}
\end{table*}
