# Supplementary material for: $\sigma$-zero: Gradient-based Optimization of $\ell_0$-norm Adversarial Examples
Source: arXiv:2402.01879 source file (2025-03-06)
Supplement: Supplementary file 9 [file backup_full_1k_cifar.tex]

%TABLE HACKS
\aboverulesep=0.2ex
\belowrulesep=0.2ex

\begin{table*}[!htb]
\caption{Results for CIFAR10 with $N=1000$. See the caption of Table~\ref{tab:exp_results_mnist} for further details. When VFGA exceeds the VRAM limit, we re-run it using a smaller batch size, increasing its runtime $t$. We denote those cases with the symbol `$\star$'.}
\label{tab:exp_results_cifar}
\centering
\resizebox{1\textwidth}{!}{%
  \renewcommand{\arraystretch}{0.96}
\begin{tabular}{r|c|cccc|ccc|c|cccc|ccc}
\toprule
\textbf{Attack} & \textbf{M}& \textbf{ASR$_{10}$} & \textbf{ASR$_{50}$} & \textbf{ASR$_\infty$} & \medianlzero & $\mathbf{t}$ & $\mathbf{q}$  &\textbf{VRAM}& \textbf{M}& \textbf{ASR$_{10}$} & \textbf{ASR$_{50}$} & \textbf{ASR$_\infty$} & \medianlzero & $\mathbf{t}$ & $\mathbf{q}$  &\textbf{VRAM}\\ \midrule
{SF} &  & 11.19 & 11.19 & 56.56 & 3072 & 1.42 & 0.37 & 1.57 &  & 16.74 & 16.79 & 35.38 & \binfty & 19.74 & 0.62 & 10.00 \\
EAD &  & 6.74 & 21.33 & 100.0 & 126 & 2.32 & 6.90 & 1.47 &  & 14.47 & 35.90 & 100.0 & 74 & 10.76 & 5.55 & 9.92 \\
{PDPGD} &  & 16.58 & 78.97 & 100.0 & 27 & 0.64 & 2.00 & 1.31 &  & 17.68 & 40.89 & 100.0 & 69 & 3.96 & 2.00 & 8.86 \\
{VFGA} &  & 48.58 & 93.41 & 99.99 & 11 & 0.17 & 0.32 & 11.96 &  & 27.71 & 67.51 & 99.88 & 29 & 4.91$^\star$ & 1.02 & \color[HTML]{FF0000} > 40 \\
{BB} &  & 69.77 & 99.79 & 100.0 & 7 & 5.81 & 2.76 & 1.47 &  & 13.46 & 17.14 & 17.94 & \binfty & 3.46 & 2.08 & 9.93 \\
%%{\PGDlzero} &  & 31.82 & 85.21 & 100.0 & 18 & 6.46 & 1.93 & 1.73 &  & 20.45 & 50.78 & 100.0 & 48 & 19.20 & 1.92 & 10.95 \\
%%{Sparse-RS} &  & \textbf{81.30} & 99.80 & 100.0 & \textbf{4} & 3.76 & 1.49 & 1.74 &  & 41.92 & 75.63 & 100.0 & 15 & 26.35 & 2.40 & 10.90 \\
{FMN} &  & 67.52 & 99.97 & 100.0 & 7 & 0.60 & 2.00 & 1.3 &  & 27.97 & 68.38 & 100.0 & 29 & 3.91 & 2.00 & 8.86 \\
{BBadv} &  & 69.58 & 99.86 & 100.0 & 7 & 4.57 & 2.01 & 1.63 &  & 38.46 & 88.92 & 100.0 & 16 & 8.85 & 2.01 & 10.03 \\
\cdashline{1-17}
{\sigmazero} & \multirow{-10}{*}{\textit \standardshort} & \textbf{80.84} & \textbf{100.0} & 100.0 & \textbf{5} & 0.74 & 2.00 & 1.51 & \multirow{-10}{*}{\textit \gowalshort} & \textbf{48.38} & \textbf{94.47} & 100.0 & \textbf{11} & 4.41 & 2.00 & 10.43 \\ \hline
{SF} &  & 18.31 & 18.77 & 56.39 & 3072 & 11.31 & 1.40 & 1.62 &  & 23.67 & 24.85 & 62.41 & 3072 & 9.86 & 0.20 & 5.50 \\
{EAD} &  & 12.70 & 30.38 & 100.0 & 90 & 1.92 & 5.70 & 1.47 &  & 17.29 & 33.68 & 100.0 & 105 & 8.33 & 5.37 & 5.39 \\
{PDPGD} &  & 16.47 & 42.50 & 100.0 & 63 & 0.64 & 2.00 & 1.32 &  & 21.37 & 48.96 & 99.82 & 51 & 2.15 & 2.00 & 5.12 \\
{VFGA} &  & 28.98 & 75.37 & 99.92 & 24 & 0.59 & 0.78 & 11.71 &  & 34.17 & 81.79 & 99.89 & 20 & 4.30$^\star$ & 0.62 & \color[HTML]{FF0000} > 40 \\
{BB} &  & 11.73 & 14.24 & 14.70 & \binfty & 0.63 & 2.05 & 1.47 &  & 37.98 & 78.76 & 83.58 & 16 & 12.49 & 3.14 & 5.39 \\
%{\PGDlzero} &  & 21.40 & 56.85 & 100.0 & 39 & 5.79 & 1.92 & 1.75 &  & 26.38 & 65.60 & 100.0 & 30 & 28.95 & 1.89 & 6.40 \\
%{Sparse-RS} &  & 36.41 & 69.49 & 100.0 & 21 & 9.97 & 2.53 & 1.71 &  & 36.40 & 68.55 & 100.0 & 23 & 34.99 & 2.46 & 6.40 \\
{FMN} &  & 28.43 & 74.70 & 100.0 & 26 & 0.59 & 2.00 & 1.31 &  & 33.30 & 79.70 & 100.0 & 21 & 2.05 & 2.00 & 5.12 \\
{BBadv} &  & 37.64 & 90.57 & 100.0 & 16 & 4.68 & 2.01 & 1.64 &  & 43.93 & 93.42 & 100.0 & 13 & 6.99 & 2.01 & 5.51 \\
\cdashline{1-17}
{\sigmazero} & \multirow{-10}{*}{\textit \carmonshort} & \textbf{47.15} & \textbf{95.38} & 100.0 & \textbf{11} & 0.73 & 2.00 & 1.53 & \multirow{-10}{*}{\textit \chenshort} & \textbf{52.46} & \textbf{97.33} & 100.0 & \textbf{10} & 2.75 & 2.00 & 5.90 \\ \hline
{SF} &  & 14.30 & 21.22 & 98.74 & 3070 & 3.62 & 0.46 & 1.90 &  & 11.98 & 12.14 & 70.77 & 3072 & 3.28 & 0.22 & 2.25 \\
{EAD} &  & 9.21 & 11.42 & 100.0 & 360 & 2.53 & 5.62 & 1.89 &  & 9.38 & 23.62 & 100.0 & 148 & 2.23 & 5.80 & 2.15 \\
{PDPGD} &  & 13.96 & 45.15 & 100.0 & 55 & 1.12 & 2.00 & 1.8 &  & 11.97 & 38.41 & 100.0 & 69 & 0.76 & 2.00 & 2.0 \\
{VFGA} &  & 21.82 & 66.50 & 99.62 & 34 & 0.48 & 0.94 & 16.53 &  & 22.79 & 56.72 & 99.81 & 39 & 3.15$^\star$ & 1.84 & \color[HTML]{FF0000} > 40 \\
{BB} &  & 21.32 & 56.78 & 58.64 & 33 & 2.31 & 2.89 & 1.89 &  & 38.82 & 93.24 & 100.0 & 15 & 6.49 & 2.87 & 2.16 \\
%{\PGDlzero} &  & 17.33 & 58.82 & 100.0 & 39 & 10.31 & 1.93 & 2.30 &  & 16.28 & 52.21 & 100.0 & 45 & 7.14 & 1.94 & 2.59 \\
%{Sparse-RS} &  & 23.52 & 57.17 & 100.0 & 37 & 20.79 & 2.66 & 2.29 &  & 33.11 & 66.15 & 100.0 & 25 & 8.46 & 2.48 & 2.57 \\
{FMN} &  & 20.61 & 71.70 & 100.0 & 33 & 1.08 & 2.00 & 1.8 &  & 23.95 & 70.24 & 100.0 & 30 & 0.73 & 2.00 & 2.0 \\
{BBadv} &  & 31.64 & 96.31 & 100.0 & 17 & 3.92 & 2.01 & 1.99 &  & 38.13 & 92.91 & 100.0 & 15 & 6.02 & 2.01 & 2.22 \\
\cdashline{1-17}
{\sigmazero} & \multirow{-10}{*}{\textit \augustinshort} & \textbf{36.61} & \textbf{97.55} & 100.0 & \textbf{15} & 1.41 & 2.00 & 1.92 & \multirow{-10}{*}{\textit \xushort} & \textbf{47.62} & \textbf{96.93} & 100.0 & \textbf{11} & 0.89 & 2.00 & 2.65 \\ \hline
{SF} &  & 15.52 & 40.86 & 93.82 & 3039 & 9.3 & 1.56 & 1.90 &  & 23.18 & 26.54 & 51.80 & 3072 & 0.58 & 0.33 & 0.51 \\
{EAD} &  & 9.48 & 11.14 & 100.0 & 398 & 2.57 & 5.66 & 1.89 &  & 15.75 & 29.23 & 100.0 & 118 & 1.01 & 5.32 & 0.41 \\
{PDPGD} &  & 15.50 & 49.19 & 100.0 & 51 & 1.16 & 2.00 & 1.8 &  & 19.43 & 41.00 & 100.0 & 66 & 0.44 & 2.00 & 0.36 \\
{VFGA} &  & 30.50 & 90.04 & 99.88 & 19 & 0.28 & 0.52 & 16.53 &  & 29.55 & 74.15 & 99.54 & 25 & 0.17 & 0.77 & 3.07 \\
{BB} &  & 16.32 & 31.03 & 31.36 & \binfty & 3.01 & 2.37 & 1.89 &  & 38.64 & 91.83 & 100.0 & 15 & 10.90 & 2.93 & 0.41 \\
%{\PGDlzero} &  & 19.90 & 70.04 & 100.0 & 33 & 8.97 & 1.93 & 2.30 &  & 24.20 & 59.98 & 100.0 & 36 & 4.10 & 1.90 & 0.56 \\
%{Sparse-RS} &  & 24.59 & 62.26 & 100.0 & 32 & 20.6 & 2.68 & 2.29 &  & 31.85 & 59.87 & 100.0 & 31 & 5.92 & 3.95 & 0.54 \\
{FMN} &  & 26.85 & 85.60 & 100.0 & 23 & 1.09 & 2.00 & 1.8 &  & 29.75 & 73.71 & 100.0 & 26 & 0.41 & 2.00 & 0.36 \\
{BBadv} &  & 37.06 & 99.11 & 100.0 & 14 & 4.51 & 2.01 & 1.99 &  & 38.01 & 93.04 & 100.0 & 16 & 4.60 & 2.01 & 0.54 \\
\cdashline{1-17}
{\sigmazero} & \multirow{-10}{*}{\textit \engstromshort} & \textbf{42.96} & \textbf{99.15} & 100.0 & \textbf{12} & 1.39 & 2.00 & 1.91 & \multirow{-10}{*}{\textit \addepallishort} & \textbf{44.29} & \textbf{94.21} & 100.0 & \textbf{13} & 0.63 & 2.00 & 0.51 \\ \hline
{SF} &  & 15.89 & 24.36 & 58.29 & 3072 & 1.63 & 0.48 & 0.66 &  & 26.85 & 43.07 & 91.14 & 69 & 4.32 & 1.49 & 0.66 \\
{EAD} &  & 12.96 & 13.23 & 100.0 & 800 & 0.94 & 4.89 & 0.65 &  & 23.94 & 24.78 & 100.0 & 768 & 1.04 & 4.99 & 0.65 \\
{PDPGD} &  & 15.95 & 35.13 & 100.0 & 75 & 0.41 & 2.00 & 0.59 &  & 26.89 & 42.38 & 100.0 & 66 & 0.40 & 2.00 & 0.60 \\
{VFGA} &  & 18.86 & 49.98 & 99.72 & 51 & 0.32 & 1.25 & 4.44 &  & 33.61 & 69.47 & 99.83 & 28 & 0.25 & 0.82 & 4.22 \\
{BB} &  & 14.13 & 22.91 & 27.64 & \binfty & 1.04 & 2.25 & 0.65 &  & 24.72 & 27.98 & 29.50 & \binfty & 0.54 & 2.09 & 0.65 \\
%{\PGDlzero} &  & 17.05 & 36.85 & 100.0 & 72 & 4.45 & 1.92 & 0.72 &  & 28.20 & 45.42 & 100.0 & 60 & 4.44 & 1.85 & 0.70 \\
%{Sparse-RS} &  & 17.78 & 31.11 & 100.0 & 138 & 9.99 & 2.77 & 0.69 &  & 33.04 & 51.26 & 100.0 & 47 & 9.48 & 2.35 & 0.68 \\
{FMN} &  & 18.61 & 48.87 & 100.0 & 52 & 0.24 & 2.00 & 0.60 &  & 32.63 & 62.96 & 100.0 & 34 & 0.35 & 2.00 & 0.59 \\
{BBadv} &  & 19.93 & 72.43 & 100.0 & 34 & 5.28 & 2.01 & 0.64 &  & 35.67 & 82.46 & 100.0 & 22 & 3.03 & 2.01 & 0.65 \\
\cdashline{1-17}
{\sigmazero} & \multirow{-10}{*}{\textit \croceloneshort} & \textbf{21.49} & \textbf{73.02} & \textbf{100.0} & \textbf{32} & 0.43 & 2.00 & 0.71 & \multirow{-10}{*}{\textit \jiangloneshort} & \textbf{37.27} & \textbf{82.92} & 100.0 & \textbf{20} & 0.42 & 2.00 & 0.72 \\ \bottomrule
\end{tabular}
}
\end{table*}
