# Supplementary material for: $\sigma$-zero: Gradient-based Optimization of $\ell_0$-norm Adversarial Examples
Source: arXiv:2402.01879 source file (2025-03-06)
Supplement: Supplementary file 10 [file backup_full_1k_imagenet.tex]

%TABLE HACKS
\aboverulesep=0.2ex
\belowrulesep=0.2ex
\renewcommand{\arraystretch}{1.05}



\begin{table*}[htbp]
\caption{Results for Imagenet with $N=1000$. See the caption of Table~\ref{tab:exp_results_cifar} for further details.}
\label{tab:exp_results_imagenet}
\centering
\resizebox{1\textwidth}{!}{%
\begin{tabular}{r|c|cccc|ccc|c|cccc|ccc}
\toprule
\textbf{Attack} & \textbf{M}& \textbf{ASR$_{10}$} & \textbf{ASR$_{50}$} & \textbf{ASR$_\infty$} & \medianlzero & $\mathbf{t}$ & $\mathbf{q}$  &\textbf{VRAM}& \textbf{M}& \textbf{ASR$_{10}$} & \textbf{ASR$_{50}$} & \textbf{ASR$_\infty$} & $ \medianlzero $ & $\mathbf{t}$ & $\mathbf{q}$  &\textbf{VRAM}\\ \midrule
EAD &  & 34.4 & 36.3 & 100.0 & 460 & 4.13 & 2.69 & 0.46 &  & 56.2 & 61.4 & 100.0 & 0 & 7.89 & 5.29 & 0.48 \\
{VFGA} &  & 47.2 & 72.5 & 99.9 & 14 & 1.22$^\star$ & 1.08 & \color[HTML]{FF0000} > 40 &  & 61.6 & 76.6 & 99.3 & 0 & 1.74$^\star$ & 1.21 & \color[HTML]{FF0000} > 40 \\
{FMN} &  & 48.7 & 81.0 & 100.0 & 12 & 0.73 & 2.00 & 0.66 &  & 63.8 & 78.7 & 100.0 & 0 & 0.72 & 2.00 & 0.67 \\
{BBadv} &  & 55.9 & 93.2 & 100.0 & 7 & 231.67 & 2.01 & 0.72 &  & 70.4 & 89.6 & 100 & 0 & 199.47 & 2.01 & 0.73 \\
\cdashline{1-17}
{\sigmazero} & \multirow{-5}{*}{\textit \resnetvulnerableshort} & \textbf{62.0} & \textbf{95.9} & 100.0 & \textbf{5} & 1.18 & 2.00 & 0.84 & \multirow{-5}{*}{\textit \salmanshort} & \textbf{75.5} & \textbf{92.8} & 100.0 & 0 & 1.13 & 2.00 & 0.84 \\ \hline
{EAD} &  & 44.6 & 51.0 & 100.0 & 42 & 18.10 & 5.45 & 1.42 &  & 26.5 & 28.4 & 100.0 & 981 & 19.25 & 5.49 & 1.41 \\
{VFGA} &  & 49.1 & 63.4 & 96.7 & 12 & 8.21$^\star$ & 2.35 & \color[HTML]{FF0000} > 40 &  & 36.6 & 59.5 & 97.9 & 31 & 6.93$^\star$ & 1.98 & \color[HTML]{FF0000} > 40 \\
{FMN} &  & 50.9 & 67.0 & 100.0 & 9 & 1.97 & 2.00 & 2.30 &  & 38.1 & 67.7 & 100.0 & 25 & 1.98 & 2.00 & 2.30 \\
{BBadv} &  & 57.5 & 82.3 & 100 & 4 & 182.65 & 2.01 & 2.40 &  & 44.3 & 85.5 & 100.0 & 14 & 205.11 & 2.01 & 2.41 \\
\cdashline{1-17}
{\sigmazero} & \multirow{-5}{*}{\textit \engstromimagenetshort} & \textbf{63.1} & \textbf{87.4} & 100.0 & \textbf{3} & 2.75 & 2.00 & 2.52 & \multirow{-5}{*}{\textit \hendrycksshort} & \textbf{46.6} & \textbf{86.9} & 100.0 & \textbf{13} & 2.76 & 2.00 & 2.52 \\ \hline
{EAD} &  & 55.1 & 60.2 & 100.0 & 0 & 21.38 & 5.50 & 1.41 &  & 32.3 & 33.5 & 100.0 & 572 & 11.43 & 5.34 & 1.68 \\
{VFGA} &  & 62.2 & 76.2 & 98.8 & 0 & 6.11$^\star$ & 1.43 & \color[HTML]{FF0000} > 40 &  & 35.4 & 46.5 & 95.5 & 66 & 33.88$^\star$ & 3.97 & \color[HTML]{FF0000} > 40 \\
{FMN} &  & 64.1 & 79.5 & 100.0 & 0 & 1.97 & 2.00 & 2.30 &  & 35.6 & 47.2 & 100.0 & 58 & 4.28 & 2.00 & 2.97 \\
{BBadv} &  & 72.4 & 89.0 & 100.0 & 0 & 185.34 & 2.01 & 2.41 &  & 38.8 & 59..8 & 100.0 & 31 & 178.06 & 2.01 & 3.07 \\
\cdashline{1-17}
{\sigmazero} & \multirow{-5}{*}{\textit \wongshort} & \textbf{75.5} & \textbf{91.4} & 100.0 & 0 & 2.76 & 2.00 & 2.52 & \multirow{-5}{*}{\textit \debenedettishort} & \textbf{40.7} & \textbf{65.1} & 100.0 & \textbf{23} & 5.72 & 2.00 & 3.20 \\ \bottomrule
\end{tabular}


    }
\end{table*}
