# Supplementary material for: $\sigma$-zero: Gradient-based Optimization of $\ell_0$-norm Adversarial Examples
Source: arXiv:2402.01879 source file (2025-03-06)
Supplement: Supplementary file 11 [file backup_full_1k_mnist.tex]

%TABLE HACKS
\aboverulesep=0.2ex
\belowrulesep=0.2ex
\renewcommand{\arraystretch}{1}

\begin{table*}[t]
\caption{Results on MNIST with $N=1000$. For each attack and model ({M}), we report ASR at $k=10, 50, \infty$, median perturbation size \medianlzero, mean runtime $t$ (in seconds), mean number of queries $q$ ($\div$ 1000), and maximum VRAM usage (in GB).}
\label{tab:exp_results_mnist}
\centering
\resizebox{1\textwidth}{!}{%
\begin{tabular}{r|c|cccc|ccc|c|cccc|ccc}
\toprule
\textbf{Attack} & \textbf{M}& \textbf{ASR$_{10}$} & \textbf{ASR$_{50}$} & \textbf{ASR$_\infty$} & \medianlzero & $\mathbf{t}$ & $\mathbf{q}$  &\textbf{VRAM}& \textbf{M}& \textbf{ASR$_{10}$} & \textbf{ASR$_{50}$} & \textbf{ASR$_\infty$} & \medianlzero & $\mathbf{t}$ & $\mathbf{q}$  &\textbf{VRAM}\\ \midrule
{SF} &  & 4.86 & 6.76 & 96.98 & 469 & 1.07 & 0.18 & 0.06 &  & 0.93 & 1.21 & 91.68 & 463 & 2.87 & 0.86 & 0.07 \\
EAD &  & 1.14 & 53.66 & 100.0 & 49 & 0.47 & 6.28 & 0.05 &  & 1.20 & 55.57 & 100.0 & 48 & 0.50 & 6.73 & 0.05 \\
{PDPGD} &  & 2.97 & 74.08 & 100.0 & 38 & 0.23 & 2.00 & 0.04 &  & 3.31 & 66.30 & 100.0 & 42 & 0.23 & 2.00 & 0.04 \\
{VFGA} &  & 9.62 & 82.42 & 99.98 & 27 & 0.05 & 0.77 & 0.21 &  & 1.80 & 39.33 & 99.95 & 57 & 0.05 & 1.33 & 0.21 \\
{BB} &  & 14.97 & 97.86 & 100.0 & 18 & 0.90 & 2.99 & 0.05 &  & 25.95 & 91.62 & 100.0 & 18 & 0.74 & 3.71 & 0.05 \\
%{\PGDlzero} &  & 12.22 & 99.84 & 100.0 & 19 & 1.15 & 1.99 & 0.07 &  & 5.04 & 90.17 & 100.0 & 24 & 1.42 & 2.00 & 0.06 \\
%{Sparse-RS} &  & 12.57 & 83.74 & 100.0 & 25 & 4.55 & 3.05 & 0.07 &  & 59.73 & 98.59 & 100.0 & 9 & 3.53 & 2.44 & 0.06 \\
{FMN} &  & 7.29 & 93.74 & 100.0 & 29 & 0.21 & 2.00 & 0.04 &  & 10.86 & 91.84 & 99.41 & 24 & 0.22 & 2.00 & 0.04 \\
{BBadv} &  & 14.81 & 91.23 & 100.0 & 19 & 0.77 & 2.01 & 0.07 &  & 14.42 & 40.88 & 100.0 & 89 & 0.71 & 2.01 & 0.07 \\
\cdashline{1-17}
{\sigmazero} & \multirow{-10}{*}{\textit{\smallcnnddnshort}} & \textbf{19.60} & \textbf{99.98} & 100.0 & \textbf{16} & 0.31 & 2.00 & 0.04 & \multirow{-10}{*}{\textit{\smallcnntradesshort}} & \textbf{61.57} & \textbf{100.0} & 100.0 & \textbf{9} & 0.31 & 2.00 & 0.04 \\ 
\bottomrule
\end{tabular}
}
\end{table*}
